# Supplementary material for: Real-space characterization of cavity-coupled waveguide systems in hypersonic phononic crystals
Source: arXiv:1909.04827 source file (2019-09-11)
Supplement: Supplementary file 1 [file Suppl_mater_v2.pdf]

# Supplementary Material

## Real-space characterization of cavity-coupled waveguide systems in hypersonic phononic crystals

D. Hatanaka,* and H. Yamaguchi

*NTT Basic Research Laboratories, NTT Corporation, Atsugi-shi, Kanagawa 243-0198, Japan*

## 1 Rayleigh wave and Lamb wave

The PnC device structure is composed of two parts: bulk joint parts and a suspended membrane, as shown in Fig. S1(a). Acoustic waves excited from one IDT formed on the GaAs bulk part propagate on the surface of the bulk and this is called Rayleigh wave as shown in Fig. S1(b). When the waves arrive at the suspended membrane containing a PnC lattice, they are transformed into Lamb waves and propagate in the membrane as shown in Fig. S1(b). Figure S1(c) shows the spatial evolution of the acoustic wave transmission in a line-defect PnC waveguide at 0.4861 GHz. The excited acoustic waves are injected as Rayleigh waves from the bulk part (0-20 $\mu$m) and then, propagate in the membrane (20-100 $\mu$m). The acoustic wavelength changes from the bulk to membrane parts because of the dispersion relation mismatch between Rayleigh and Lamb waves.

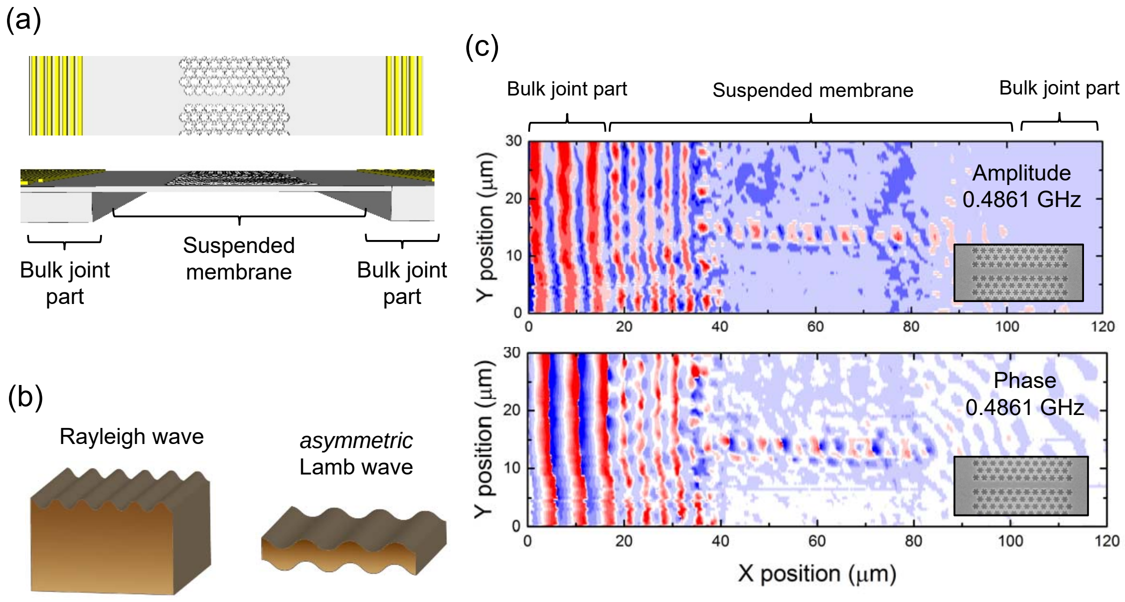


Figure S1: (**a**) Schematics of a PnC device in which a PnC membrane is suspended by bulk joint parts. (**b**) Schematic of a Rayleigh wave (left) and an asymmetric Lamb wave (right). (**c**) Real-space mapping of the amplitude (top) and phase (bottom) of acoustic waves at 0.4861 GHz. A line-defect waveguide is formed in a PnC lattice with dimensions $a = 4.0$ $\mu$m, $b = 3.5$ $\mu$m, $w = 1.0$ $\mu$m and $t = 0.9$ $\mu$m as shown in the insets.

## 2 L1, L3 and L4 cavities

Figures S2(a)-(c) show experimentally-obtained $Q$ factors as function of resonant frequency in L1, L3 and L4 cavities, respectively. Multiple resonant hypersonic vibrations are also observed at 0.50-0.58 GHz in these cavities. All the modes are experimentally identified by the real-space mapping technique as shown in Fig. S3. In particular, additional modes M6-M8 are found in the L3 and L4 cavities. The resonant frequencies calculated by FEM using the anisotropic elastic parameters are shown as solid lines.

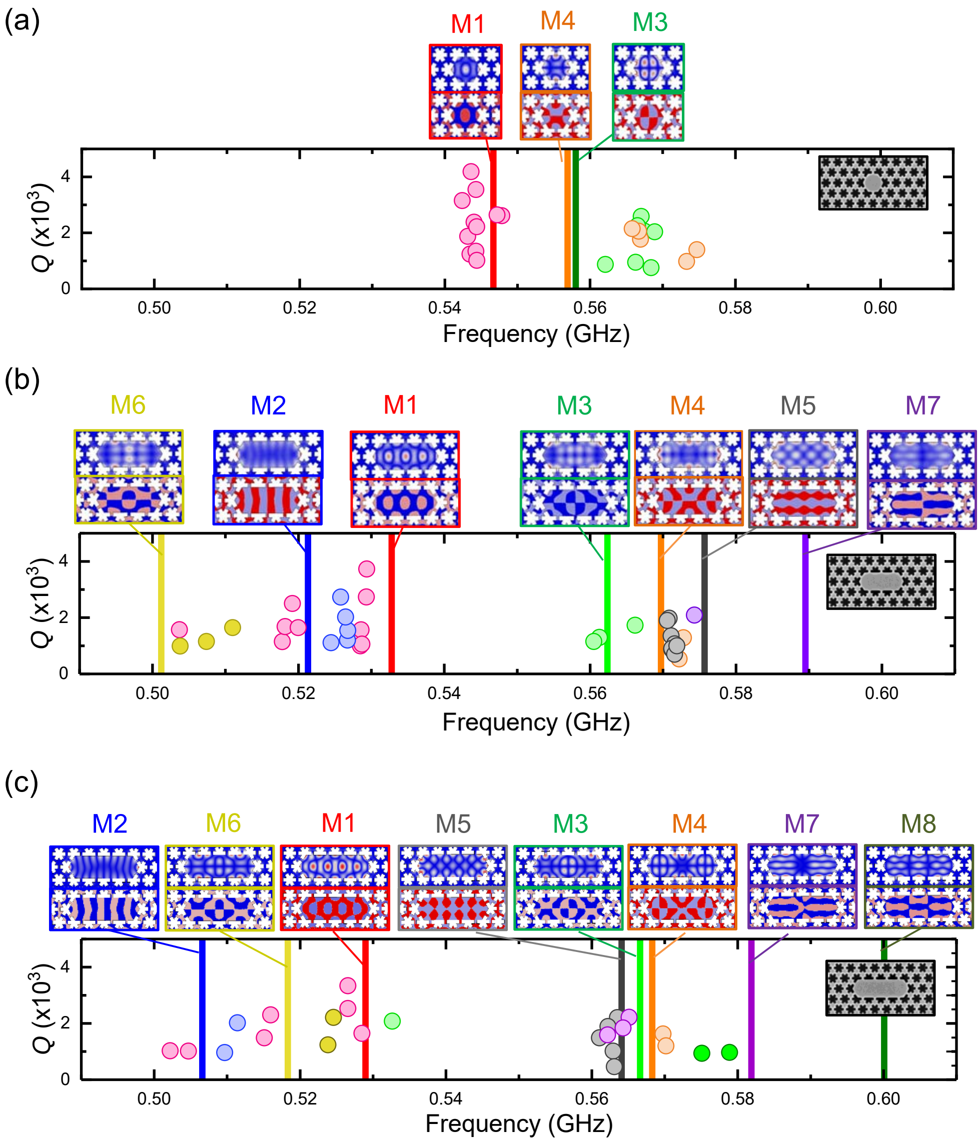


Figure S2: **(a)-(c)** $Q$ factors as a function of resonant frequency in various vibration modes in L1, L3 and L4 cavities with $N$ = 5-7, respectively. The corresponding mode profiles obtained by FEM are shown in the top panels.

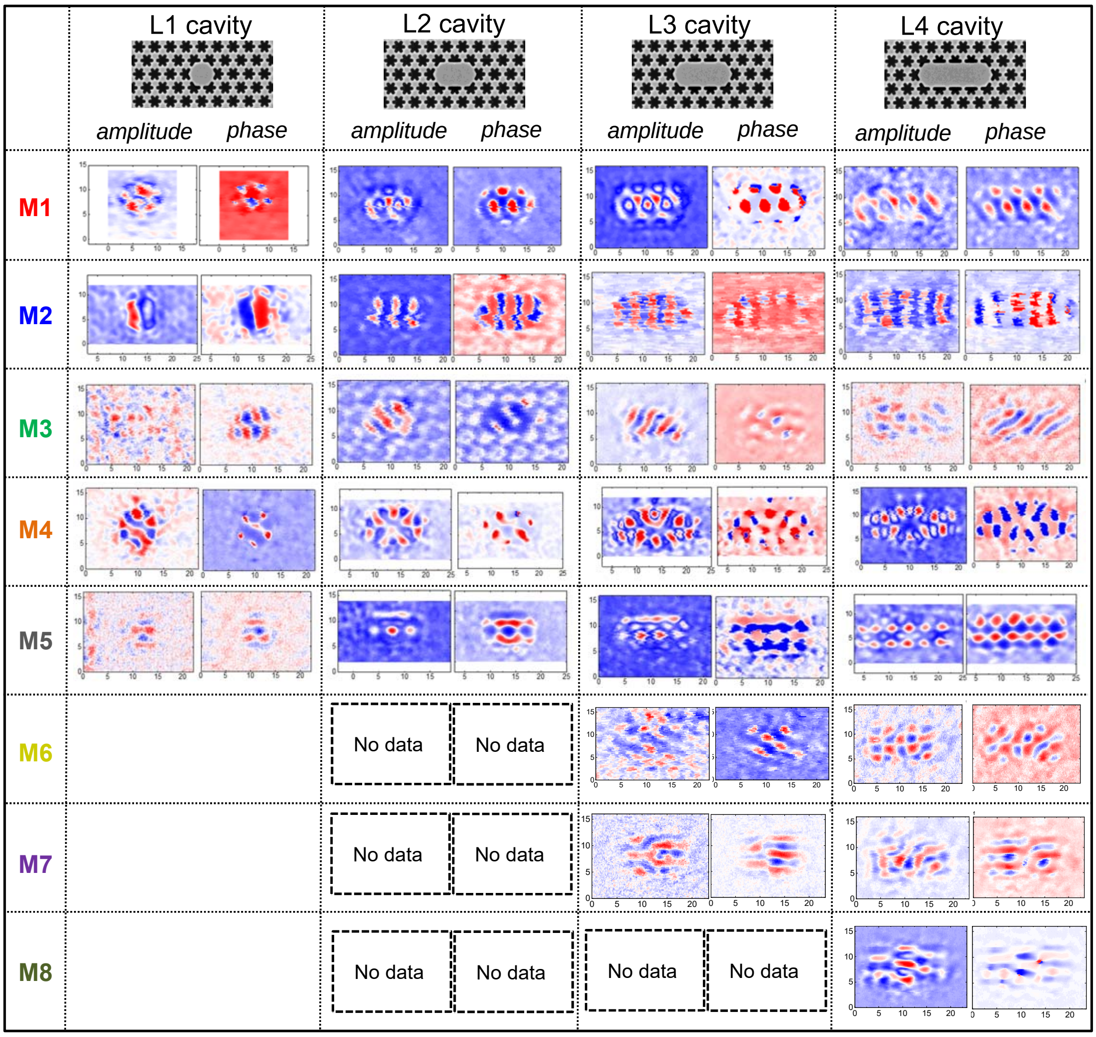


Figure S3: The amplitude and phase distribution of various modes in L1-L4 cavities. The M2 mode in an L1 cavity is experimentally identified around 0.525 GHz, but not in FEM. M6-M8 modes are not predicted in an L1 cavity by FEM. The M5 mode in an L1 cavity, which is not shown in Fig. S2, is only observed with $N = 2$ at 0.582 GHz. The calculations also show M6-M8 modes in an L2 cavity and M8 mode in an L3 cavity, but they are not found experimentally in the frequency range 0.50-0.58 GHz.

# 3 Effects of PnC shield and thermoelastic damping on $Q$ factor

The effects of a phononic bandgap (BG) and thermoelastic damping (TED) on the $Q$ factor are investigated by designing an L1 PnC cavity with FEM calculations as shown in Fig. S4(a) and S4(b). The $Q$ value of the M1 mode greatly increases with the period number ($N$) when we only consider the BG effect, and it achieves $> 10^{13}$ at $N > 4$ as shown by the green line in Fig. S4(c). However, the introduction of the TED effect into the simulation causes $Q$ to saturate around $10^4$ at $N \geq 2$. The remaining difference between the simulated $Q$s and the experimental values can be the result of other internal dissipation sources such as TLS, which is not included in the FEM. As reported for GaAs optomechanical systems [M. Hamoumi et al, Phys. Rev. Lett. **120**, 223601 (2018).], TLS is a key factor to determining $Q$ in GaAs mechanical devices at room temperature. Thus, the FEM results indicate that the energy dissipation in a cavity with a PnC shield $N \geq 2$ is mainly determined by these internal dissipation sources and this is also reasonable as regards to the experimental results in Fig. 5.

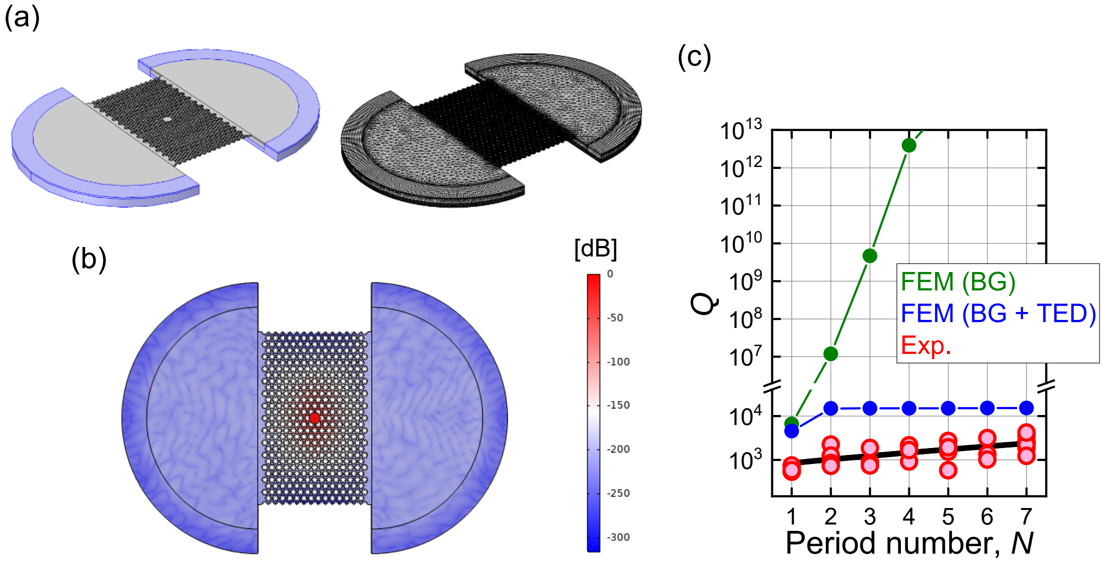


Figure S4: **(a)** Design of an L1 Pnc cavity in FEM simulations (left) where perfectly matched layers are introduced to avoid undesired reflection as denoted by blue. A dense mesh is inserted into the structure (right). **(b)** Mechanical energy field profile of the M1 mode in an L1 cavity, in which the PnC shield strongly suppresses the energy dissipation to the bulk joint parts. **(c)** $Q$ factors of the M1 mode in L1 cavities as a function of $N$, which are experimentally obtained (red) and FEM simulated by including the BG and TED effects (blue) and only the BG effect (green).
